# Supplementary material for: Learning Locally Editable Virtual Humans
Source: arXiv:2305.00121 source file (2023-04-28)
Supplement: Supplementary file 1 [file FIG_2D.tex]

\begin{figure*}[t]
\centering
\includegraphics[width=\linewidth]{images/2d.pdf}
\caption{\textbf{More personalized texture editing results}. We draw customized textures on 2D images and fit avatars' texture features. Note that these local textures remain consistent under pose changes.}
\label{fig:2D}
\end{figure*}
